# Supplementary material for: Chaos persists in large-scale multi-agent learning despite adaptive learning rates
Source: arXiv:2306.01032 source file (2026-10-17)
Supplement: Supplementary file 1 [file App-Test.tex]

%----------------------------------------------------------------------
%%% APP: TEST
%----------------------------------------------------------------------
% !TEX root = ../Main.tex

This is a test appendix.
A test equation follows below:
\begin{equation}
\pay_{\play}(\strat)
	= \sum_{\pure_{\play}\in\pures_{\play}}
		\sum_{\pure_{-\play}\in\pures_{-\play}}
		\strat_{\play\pure_{\play}}
		\strat_{-\play\pure_{-\play}}
		\pay_{\play}(\pure_{\play};\pure_{-\play})
\end{equation}
